# Supplementary material for: Lowering qubit requirements for quantum simulations of fermionic systems
Source: arXiv:1712.07067 source file (2018-10-11)
Supplement: Supplementary file 1 [file ArticleQ_suppl.pdf]

# Manual for the supplementary Mathematica program

Mark Steudtner[1, 2] and Stephanie Wehner[2]

[1] Instituut-Lorentz, Universiteit Leiden, P.O. Box 9506, 2300 RA Leiden, The Netherlands
[2] QuTech, Delft University of Technology, Lorentzweg 1, 2628 CJ Delft, The Netherlands

(Dated: December 19, 2017)

## I. PURPOSE

Provided by this small Mathematica code is a tool to transform Hamiltonians of the form

$$H = \sum_{l=0}^{\infty} \sum_{\substack{\boldsymbol{a}\in[N]^{\otimes l} \\ \boldsymbol{b}\in\mathbb{Z}_2^{\otimes l}}} h_{\boldsymbol{ab}} \prod_{i=1}^{l} (c_{a_i}^{\dagger})^{b_i} (c_{a_i})^{1+b_i \bmod 2}$$
$$= \sum_{l} \sum_{\substack{\boldsymbol{a},\boldsymbol{b} \\ \text{with } h_{\boldsymbol{ab}}\neq 0}} \hat{h}_{\boldsymbol{ab}} \,, \tag{1}$$

into Hamiltonians of the form

$$\mathsf{H} \;=\; \sum_{\sigma\in\{X,Y,Z,\mathbb{I}\}^{\otimes n}} \theta_\sigma \times \sigma \qquad \text{with all} \quad \theta_\sigma \in \mathbb{R} \,, \tag{2}$$

using binary codes. We explicitly allow for decoding functions $\boldsymbol{d}$ that are non-linear, but restrict ourselves to linear encodings. We furthermore decompose any controlled gates, where these may occur.

## II. BINARY FUNCTIONS

In general we need reserve the function `w` inside the program, but leave it undefined. This function represents binary variables $\omega_i$ through `w[i]`, which the Mathematica kernel does not evaluate, as it is not defined. A decoding function $\boldsymbol{d} : \boldsymbol{\omega} \to \boldsymbol{d}(\boldsymbol{\omega})$ is then defined by a list `d`, where the $i$-th element `d[[i]]` represents the component $d_i$. These components are non-linear binary functions, that we express in their analytic form, acting on the vector $\boldsymbol{\omega}$.
Let us consider an example: the decoding

$$\boldsymbol{d} : \mathbb{Z}_2^{\otimes 2} \to \mathbb{Z}_2^{\otimes 3} \,, \qquad \boldsymbol{d}(\boldsymbol{\omega}) = \begin{pmatrix} \omega_1 \\ \omega_2 \\ 1+\omega_1+\omega_2 \end{pmatrix} \bmod 2 \tag{3}$$

will be expressed as

$$\mathtt{d} = \{\mathtt{w}[1], \mathtt{w}[2], \mathtt{w}[1] + \mathtt{w}[2] + 1\} \,. \tag{4}$$

It is understood by the algorithm that the expression is always mod 2. As we for the moment only allow linear encodings, we store those in form of matrices, or to be more precise: we store one encoding matrices $A$ as lists

$$\{\{A_{11}, A_{12}, A_{13}, \ldots, A_{1N}\}, \{A_{21}, \ldots, A_{2N}\}, \ldots, \{A_{N1}, \ldots, A_{NN}\}\} \,. \tag{5}$$

The encoding of the odd Checksum code,

$$\boldsymbol{e}(\boldsymbol{\nu}) = \left[\begin{smallmatrix} 1 & 0 & 0 \\ 0 & 1 & 0 \end{smallmatrix}\right] \boldsymbol{\nu} \bmod 2 \tag{6}$$

is for for instance stored as

$$\{\{1, 0, 0\}, \{0, 1, 0\}\} \,. \tag{7}$$

## III. MAIN ROUTINE

The heart of this is the routine `transform`, that takes a Hamiltonian (1), as well as the encoding and decoding function as arguments.

$$\texttt{transform}[\mathsf{a},\mathsf{DEC},\mathsf{ENCmtx}]$$

$\mathsf{a}\ldots$ Hamiltonian of the form (8).

$\mathsf{DEC}\ldots$ decoding function in the same format as (4).

$\mathsf{ENCmtx}\ldots$ linear encoding as a mathematica array.

The output of this routine is a multinomial that corresponds to the Hamiltonian (2). Instead of the tensor product notations, e.g. $Y_2 \otimes X_5$, we will find product of the undefined functions `X`, `Y` and `Z`. This yields `X[5] Y[2]` for our example as Mathematica orders unknown functions alphabetically.

Let us now focus on the format of the input. The binary functions $\boldsymbol{d}$ and $\boldsymbol{e}$ are to be plugged-in in the format explained in the previous section. The input Hamiltonian has to be put into list form. For all contributing terms $\hat{h}_{\boldsymbol{ab}}$ with length $l$, we add an entry

$$\{(-1)^{1+b_1}a_1,\, (-1)^{b_2+1}a_2,\, \ldots\, ,\, (-1)^{b_l+1}a_l,\, h_{\boldsymbol{ab}}\} \tag{8}$$

to that list. Let us consider a minimal example. We want to use the odd Checksum code on 3 orbitals, as it is given by (6) and (3), on the Hamiltonian

$$\frac{1}{2}\left(c_1^\dagger c_3 + c_3^\dagger c_1\right)\, . \tag{9}$$

We therefore let Mathematica compute

$$\texttt{transform}[\{\{1,-3,.5\},\{3,-1,.5\}\},\{\mathsf{w}[1],\mathsf{w}[2],1+\mathsf{w}[1]+\mathsf{w}[2]\},\{\{1,0,0\},\{0,1,0\}] \tag{10}$$

which (probably after using `Chop`) yields `0.25X[1] + 0.25X[1]Z[2]`. The resulting Hamiltonian is thus $\frac{1}{4}(X_1 + X_1 \otimes Z_2)$. In the following, we explore the structure of the main routine, including explanations on the subroutines used. In another example, let us transform the creation operator $c_8^\dagger$ via the Jordan-Wigner transform. For that purpose we will use the predefined Jordan-Wigner decoding `decJW`, which takes the integer orbital number as parameter and Mathematica's identity matrix as an encoding. After typing:

$$\texttt{transform}[\{\{8,1\}\},\texttt{decJW}[10],\texttt{IdentityMatrix}[10]]\, , \tag{11}$$

we are provided with the correct result:

$$\texttt{0.5X[8]Z[1]Z[2]Z[3]Z[4]Z[5]Z[6]Z[7]} - (0. + 0.5\texttt{I})\texttt{Y[8]Z[1]Z[2]Z[3]Z[4]Z[5]Z[6]Z[7]}\, . \tag{12}$$

### A. Structure and subroutines

For a contributing Hamiltonian term $\hat{h}_{\boldsymbol{ab}}$, we need to compute the function

$$\underbrace{\left(\bigotimes_{i=1}^{n} (X_i)^{\sum_j A_{ij} q_j \bmod 2}\right)}_{(i)} \underbrace{\left(\prod_{v=1}^{l-1}\prod_{w=v+1}^{l} (-1)^{\theta_{a_v a_w}}\right)}_{(ii)} \prod_{x=1}^{l} \underbrace{\frac{1}{2}\left(\mathbb{I} - \left[\prod_{y=x+1}^{l} (-1)^{\delta_{a_x a_y}}\right] (-1)^{b_x}\, \mathfrak{X}\left[d_{a_x}\right]\right)}_{(iii)} \underbrace{\mathfrak{X}\left[p_{a_x}\right]}_{(iv)}\, . \tag{13}$$

Part $(i)$ is easily obtained as a product of the functions `X` and $(ii)$ is essentially just a number $\pm 1$ that is straightforward to calculate. For $(iv)$ we obtain the parity codes by summing components of the decoding function accordingly. In order to simplify the expressions, we apply Mathematica's pattern matching algorithm on a list of binary rules in the subroutine `binrules`, which for instance implements $2\omega_j \to 0$ and $(\omega_j)^2 \to \omega$. The treatment of $(iii)$ and $(iv)$ is very similar from there on. We implement the extraction superoperator $\mathfrak{X}$, by submitting its arguments to a pattern matching procedure with the list `extractor`. Before we can do that however, the binary functions to extract have to be subjected to the undefined function `binfun`. Applying the rules `extractor` firstly separates sums in the binary function, so for

instance transforms $\texttt{binfun}[1 + \texttt{w}[1] + \texttt{w}[1]\texttt{w}[2]] \rightarrow \texttt{binfun}[1]\texttt{binfun}[\texttt{w}[1]]\texttt{binfun}[\texttt{w}[1]\texttt{w}[2]]$. Next, all the constant terms are transformed to minus signs and all the weight-1 terms to $Z$-operators, so $\texttt{binfun}[1]\texttt{binfun}[\texttt{w}[1]]\texttt{binfun}[\texttt{w}[1]\texttt{w}[2]] \rightarrow -\texttt{Z}[1]\texttt{binfun}[\texttt{w}[1]\texttt{w}[2]]$. In the last step, the remaining terms are submitted to the subroutine `dissolve`, which implements the extraction rule for non-constant terms

$$\mathfrak{X}\left[\boldsymbol{\omega} \rightarrow \prod_{j \in \mathcal{S}} \omega_j\right] = \mathbb{I} - 2 \prod_{j \in \mathcal{S}} \frac{1}{2} \left(\mathbb{I} - Z_j\right) . \tag{14}$$

We now fuse the terms (*iii*) and (*iv*) with the expressions (*i*) by a last round of pattern matching inside the subroutine `pauliaction`. At that point, we are lucky to have the Pauli-$X$ operators on the left-hand side of the $Z$-operator, so we do not need to teach Mathematica about the algebra of those operators. We simply cancel $Z$-operators like $\texttt{Z}[1]^2 \rightarrow \texttt{1}$, and are then free to just replace $X$- and $Z$-operators by $Y$-operators analogously to $\texttt{X}[2]\texttt{Z}[2] \rightarrow -\texttt{IY}[2]$, where `I` is the imaginary unit in Mathematica. After this procedure is done for all terms in the Hamiltonian, all imaginary terms will cancel.
